# Supplementary material for: Open Source Variational Quantum Eigensolver Extension of the Quantum Learning Machine (QLM) for Quantum Chemistry
Source: arXiv:2206.08798 ancillary file (2022-11-28)
Supplement: Supplementary file 1 [file Supplementary_Materials-v2.pdf]

# Supplementary Materials: Open Source Variational Quantum Eigensolver Extension of the Quantum Learning Machine (QLM) for Quantum Chemistry

This Supplementary Materials document is organized as follows:
- In Section S1, we shed some light on the interoperability of myQLM circuits with other packages such as Qiskit, projectQ, pyQuil, Cirq...Indeed, as mentioned in Section 3 of the main text, interoperability is among of the key advantages of the myQLM library. We also provide an example on how to use interoperability features withing the OpenVQE package.
- In Section S2, we provide numerical simulations on several molecules using OpenVQE modules. These additional results complement the Section 5 of the main text.

In particular, in Subsection S2A, we first focus on the $H_6$ molecule in a single geometrical arrangement. The goal here is to study the behaviours of the different optimizers (see *scipy.optimize*, main text) in term of chemical accuracy. We also investigate how many CNOT gates are required for each of the optimizers to achieve chemical accuracy using the UCCSD method. The different choices for the initial wavefunction are also detailed (the random guess, Møller-Plesset wavefunction at second order...).

In Subsection S2B, we extend our calculations to a larger set of molecules using the STO-3G basis set. Some computations use a full space and some others include active space selections, in order to compare the chemical accuracy obtained from the regular UCCSD and QUCCSD ansätze. We then compare the results with those obtained from CCSD, CCSD(T), CISD and CIPSI classical methods. CIPSI or Configuration Interaction using a Perturbative Selection made Iteratively is a particular CI approach that uses a truncation of the Full Configuration Interaction (FCI) wave-function where the determinants are selected regarding a perturbative selection. The method has been developed since a few decades (see some references in the introduction of [1]) and it is well described in [2, 3].

In subsection SC, using the fermionic-ADAPT-VQE sub-module, we simulated several molecules using a large number of qubits (22 qubits) and different basis sets assuming full space selection. Using the same sub-module we also tested several molecules with active space selections to compare the efficiency of fermionic-ADAPT-VQE in the context of such active space approximations.

Finally, in subsection SD, we describe how the Qubit-ADAPT-VQE sub-module works through choosing different types of qubit pools associated to different size. To do so, we study the $H_4$ molecule using STO-3G basis set.

## 1. INTEROPERABILITY OF OPEN-SOURCE PACKAGES WITH MYQLM

myQLM library[4, 5] provides binders to connect with the other Python-based quantum frameworks. The role of these binders is to: (i) translate myQLM circuits into a format defined in another quantum framework and vice-versa. (ii) execute a job using a QPU defined in another quantum framework directly in myQLM and vice-versa. This is helpful to any problem in quantum computing.

When it comes to our domain of treating quantum chemistry problems using variational quantum algorithms, it is important to use myQLM tools to translate a defined wavefunction represented by a QLM circuit into Qiskit, Cirq, PyQuil etc. (See circuit translations in Fig. S1). This interoperability bridges the gap between the chemists who work in myQLM softwares and those who work on the other packages. This consequently allows them to validate their calculations, to test their algorithms and codes. Such an exchange between packages works easliy for the user by just using few lines of codes developed by myQLM package (see snippet codes shown in section 3.2 in the main text). To describe the QLM-Qiskit circuits switching using myQLM keys, we provide

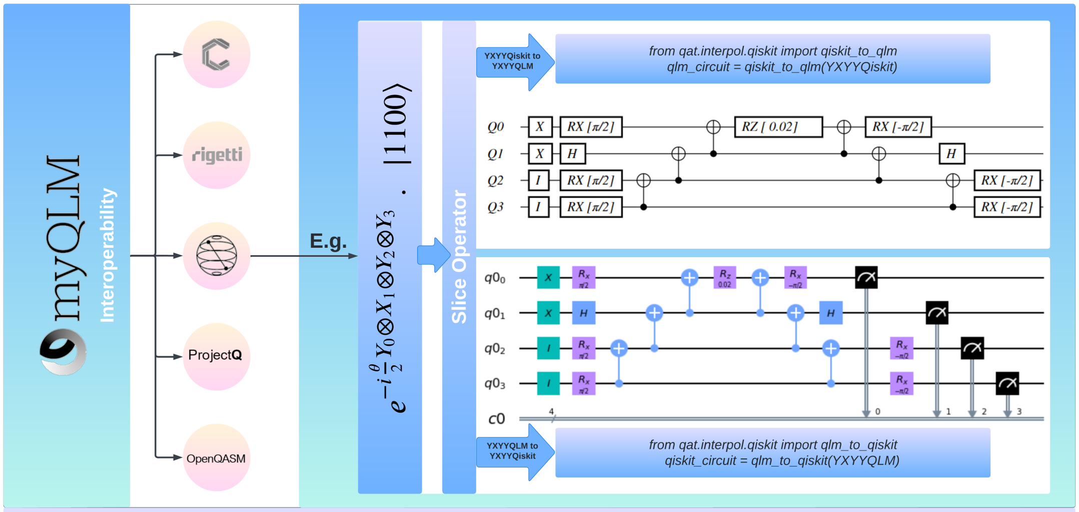


| FrameWork | | Qiskit | OpenQasm | PyQuil(no py 3.6) | Project Q | Cirq |
|---|---|---|---|---|---|---|
| Circuit translation | to QLM | Yes | Yes | Yes | Yes | Yes |
| | From QLM | Yes | No | Yes | No | Yes |
| QPU connection | to QLM | Yes | N/A | Yes | No | No |
| | From QLM | Yes | | No | No | No |

**Fig. S1.** Interoperability packages with myQLM. YXYYQLM (top circuit) and YXYY (bottom circuit). These circuits consists of 4 qubits that represents $e^{\theta Y_0\otimes X_1\otimes Y_2\otimes Y_3}|1100\rangle$, with $\theta$ is equal to 0.01.

a simple example related to qubit-ADAPT-VQE which we developed in OpenVQE package. This hopefully will make the image of myQLM interoperability clearer to the reader. As is known, qubit-ADAPT-VQE is based on pool of excitations consisting of Pauli strings that can be added adaptively step by step to construct the final ansatz. Suppose our pool consist of the $YXYY$ strings. Then mapping the exponential of each of these strings associated with their parameters into a circuit can be done typically by using CNOTstair case method[6–8]. myQLM-fermion tools can help to slice this exponential to construct this circuit, which we name it here "YXYYQLM", this construction is shown in Figure S1. By using the keys of myQLM listed in the same figure, the user can switch between YXYYQLM and YXYYQiskit immediately. We can also connect between myQLM QPU and Qiskit Backend when we want to execute a job and obtain an estimated energy. This QPU connection between packages is also shown in FigureS1.

Additionally, such interoperability feature can facilitate the user execution of a circuit on a real quantum device as shown in Figure S2. The user simply needs: i) to declare his IBM token, (ii) to

wrap a Qiskit backend in a QPU, (iii) to use a job class in order to send the circuit to a QPU to obtain the results.

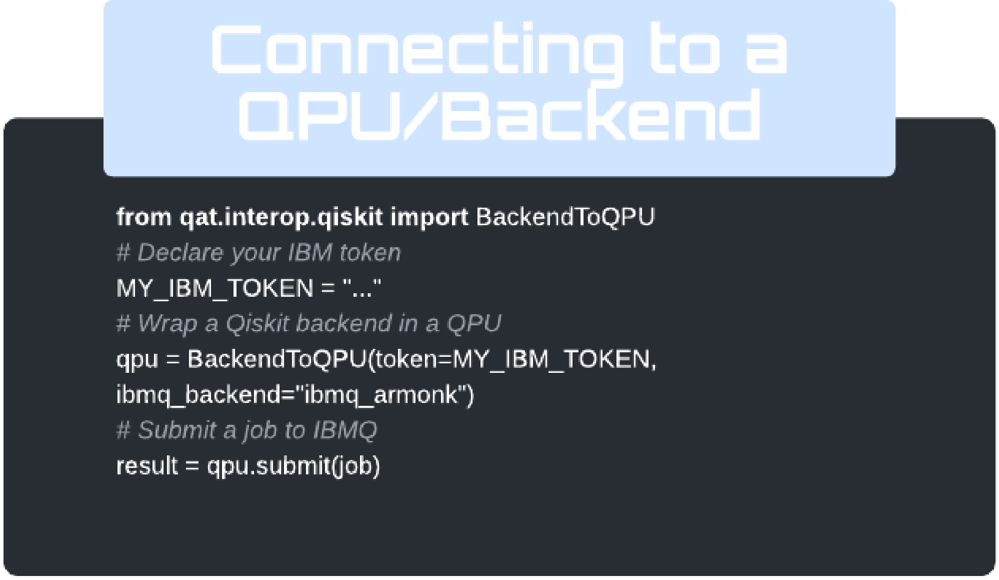


**Fig. S2.** myQLM keys: running on IBM quantum computer

## 2. FURTHER APPLICATIONS OF THE OPENVQE PACKAGE

### A. Influence of the Optimization Method on the UCCSD-VQE Performances for $H_6$ molecule, r=1.0 Å

After showing the performance of the UCCSD-VQE sub-module in terms of active space selection and MP2 pre-screening approaches in subsection 5.2 in the main text. Here we aim to test further the usefulness of using MP2 guesses in VQE-UCC algorithm. To do this, We choose the $H_6$ molecule associated to the STO-3G basis set at a bond length of $r = 1.0$Å using a full space. We calculated UCCSD-VQE energies using six different optimizers, namely COBYLA, BFGS, SLSQP, CG, Powell and Nelder-Mead and with three different initial guesses: (i) random, where random values are chosen uniformly in the interval $[0.0, 1.0]$; (ii) fixed-value of 0.001; (iii) MP2 guesses. In Figure S3, we compare the effects of these initial guesses on the VQE optimization based on three criteria: (i) the number of function evaluations required for convergence, see Figure S3(a); (ii) the error in the energy evaluation which corresponds to the VQE energy subtracted from the FCI energy solution, see Figure S3(b); (iii) the number of CNOT gates needed for completing a circuit after the final optimization, see Figure S3(c). From Figure S3(a) we observe that the COBYLA and Nelder-Mead methods require a high number of function evaluation ($> 30000$) to reach good VQE performances when the parameters are randomly chosen. Conversely, the other optimizers (BFGS, SLSQP, CG and Powell) requirements appear smaller. They provide less function evaluations (about 3000 up to 10000) in order to reach convergence. In practice, the Nelder-Mead approach is clearly not adapted to this case as it exhibits high energy errors ranging beyond 0.1 Ha (see Figure S3) (b).The COBYLA method appear to reach a better accuracy than SLSQP, which nevertheless requires a smaller number of function evaluations. COBYLA is known to have a better ability to explore the energy than SLSQP. The other optimizers, i.e. BFGS, CG and Powell bring comparable results between $10^{-1}$ and $10^{-2}$ Ha. On the other hand, for the 0.001 fixed-value and MP2 initial guesses methods- COBYLA, BFGS, SLSQP, CG and Powell converge well to almost the same accuracy under than $10^{-3}$ Ha.

In general, the number of evaluation changes depending on the type of optimizer: some of them require the estimation of the gradients (BFGS, SLSQP and CG) and some belong to the class

of gradient-free optimizers (COBYLA, Powell, Nealder-Mead). From Figure S3, (a) it is clear that gradient-based optimizers (BFGS, SLSQP and CG) require less function evaluations compared to gradient-free ones (COBYLA, Powell, Nealder-Mead). This is true for every optimizer and choice of initial parameters except for the "random" choice where the Powell optimizer requires less function evaluations as compared to SLSQP and BFGS. We hypothesise that this behaviour is due to the fact that the random guess of the initial parameters was closer to the optimum when the Powell optimizer was used. However, this advantage in using gradient-based (versus gradient-free) optimizers might not remain when executing algorithms on actual hardware where shot noise, relaxation and dephasing randomize the optimization landscape, making the estimation of gradients, especially fine ones, more challenging. The energy error follows a somewhat similar trend (subfigure (b)). Figure S3(c) shows that by using the `count()` function of the OpenVQE package, MP2 guesses lead to reduce the CNOT gates counts in the final circuit when using BFGS, SLSQP, CG and Powell methods. The CNOT gates are reduced by about half compared to COBYLA or Nelder-Mead. Moreover choosing a MP2 guess shows better reductions in CNOT gates counts when compared to random or 0.001 fixed-value guesses. In[9], similar analysis and comparisons between different optimizers and initial guesses is studied for H4 molecule, there, not only linear geometry path has been tested but also rectangular and trapezoidal paths. Showing that when MP2 guess is used, a smaller number of function evaluations is required, regardless which path of geometry is considered.

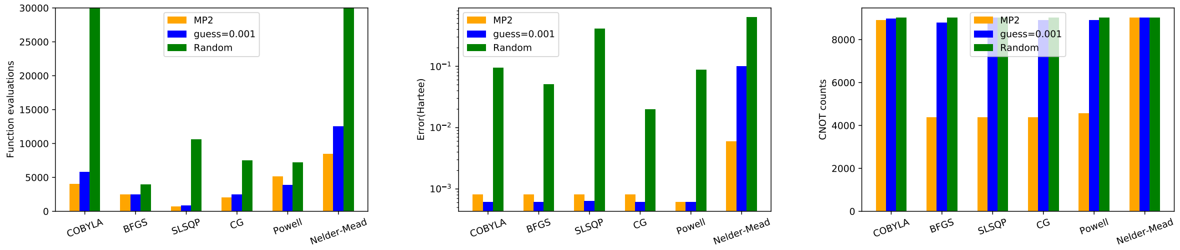


**(a)** Function evaluations **(b)** Error ground state **(c)** CNOT counts after optimization

**Fig. S3.** Basic VQE-UCCSD performances applied to the $H_6$ linear system studied using six different optimization methods (COBYLA, BFGS, SLSQP, CG, Powell and Nelder-Mead) and three distinct starting guesses for the parameters (chosen randomly from interval $[0.0, 1.0]$). (Random), all parameters were fixed at 0.001 (0.001) and used MP2 amplitudes (MP2). We compare the number of function evaluations required for convergence (Final accuracy in the optimization set as $10^{-4}$) (panel (a)), the error in the final energy with respect to the FCI energy (panel (b)), the number of CNOT gates after optimization (panel(c)). The scale of function evaluations is truncated at 30000 to enable comparisons. We remind also that we choose a tolerance of $10^{-7}$. In practice, if the parameters values appear below this condition then the operators associated to these parameters are omitted from the final UCCSD wave function.

### B. Estimation of UCCSD and QUCCSD Accuracies Compared to Classical Methods and of the Required Quantum Resources for a Range of Molecules using the STO-3G Basis Set

Following our previous discussion, we used the UCCSD and QUCCSD methods to build ansätze and chose an MP2 initial guess. We remind that UCCSD and QUCCSD circuits are implemented in OpenVQE based on the CNOT staircase method and so are QUCCSD circuits while we are using the efficient circuits introduced in [10]. The optimization is performed with the BFGS algorithm as the maximum number of function evaluations was fixed at 50,000.

To compare the resulting UCCSD and QUCCSD energies we calculated the ground state energies of the same molecules using the following four classical methods: CCSD, CCSD(T), CISD and CIPSI. The first three methods were carried out by using the Gaussian software package [11], while CIPSI computations were carried out using the Quantum Package (QP) [12] software. We also computed the FCI (for STO-3G) energy using the functions implemented in the QLM library based on the PYSCF package. We choose the following set of molecules: $H_4$, LiH, $H_6$, $BeH_2$, $H_8$,

$H_2O$ whose geometries are all near equilibrium and detailed in the `MoleculeFactory` class in $(x, y, z)$ format in OpenVQE. We choose other larger size molecules: $CH_4$, $C_2H_2$, $C_2H_4$, HCN, CO, $N_2$ and $SO_2$, which we also present in the same format in `MoleculeFactory`. We extracted the geometries of these near equilibrium larger molecules from the NIST Diatomic Spectral Database [13–16]. All these molecules we considered in a singlet ground state. Full space selections were considered for all molecules when applying CCSD, CCSD(T) and CISD techniques. However, it is not the case when we calculate UCCSD- and QUCCSD-VQE:
(i) we consider a full space selection for molecules ranging between 8 and 20 qubits, namely: $H_4$ (8 qubits), LiH (12 qubits), $H_6$ (12 qubits),$H_2O$ (14 qubits), BeH2 (14 qubits) and $H_8$ (20 qubits); (ii) we consider (AS) selection for molecules represented by more than 20 qubits due to the memory limitations of the QLM simulator in link with our computing server. So for the following molecules we choose: $CH_4$ (AS($6\eta$,$10N_A$)) i.e (10 qubits), $C_2H_2$ (AS($8\eta$,$12N_A$)) i.e (12), $C_2H_4$ (AS($4\eta$,$14N_A$)) i.e (14 qubits), HCN (AS($6\eta$,$14N_A$)) i.e (14 qubits), CO (AS($6\eta$,$12N_A$)) i.e (12 qubits), $N_2$ (AS($8\eta$,$12N_A$)) i.e (12 qubits), and $SO_2$ (AS($8\eta$,$12N_A$)) i.e (12 qubits).

In Figure S4(a), we present the results for the UCCSD and QUCCSD ansätze. These numerical values are obtained taking the absolute values of the substraction of the UCCSD and QUCCSD estimated energy from the corresponding FCI energy. As shown in Figure S4(a) Comparing ansatz performances for UCCSD to QUCCSD approaches, we observe different molecules behaviors in case of full space selections: (i) for $H_4$ and LiH, QUCCD achieves the same level of accuracy compared to the UCCSD; (ii) for $H_6$, $BeH_2$ and $H_2O$, there is a difference in the computed errors. QUCCSD performs worse than UCCSD while remaining close to chemical accuracy for these three molecules. In $H_8$, the error increased by one order of magnitude (i.e from $10^{-3}$ up to $10^{-2}$ Ha) and is above the chemical accuracy. The reason for these error variations is linked to the fact that the QUCCSD ansätze fail to recover the correlation effects that become stronger at certain bond lengths especially when the system qubit size increases (i.e. like for the 20 qubits $H_8$ system). Now for molecules within the active space selection, the QUCCSD ansatz performs as accurately as UCCSD. This means that within this size of qubits, the removal of parity terms in excitation operators may not affect the accuracy of the QUCCSD method compared to UCCSD. This is consistent with previous results obtained in reference [17] where the accuracy reached by QUCCSD was found comparable to that obtained with UCCSD for a test set of molecules including $H_4$, $H_6$, $BeH_2$, $H_2O$ and $N_2$ at similar bond lengths. Such data tend to show that despite the sole inclusion of single and double excitations, QUCCSD can approximate electronic wavefunction almost as accurately as UCCSD while not being as reliable. It can be particularly noticed in the cases of strongly correlated systems within full space ($H_8$).

Figure S4(b) displays a comparison between the CCSD, CCSD(T), CISD and CIPSI classical methods. CIPSI brings the most accurate results for all the molecules presented (by at least one order of magnitude compared to CCSD(T)). Comparing UCCSD-VQE Figure S4(a) to the classical methods displayed in Figure S4(b), we find a similar order of magnitude of error for CCSD and while better results are obtained for CISD, for $H_4$, LiH, $H_6$, $BeH_2$, $H_8$ and $H_2O$. For these molecules, the CCSD(T) approach appears as the most accurate. For molecules calculated using active space selection, we clearly find that classical methods, mainly CCSD(T) and CIPSI, bring a better accuracy since core orbitals are not frozen in these cases. Interestingly, some molecules like $C_2H_4$, CO and $SO_2$ (see Figure S4(a)) ate still able to approach the accuracy observed in classical methods such as CISD and CCSD. However CISD and CCSD are also far from the chemical accuracy reached by CCSD(T). This shows that apart from active space selection approach, the triple excitations are required for large molecules. Therefore, one would like to be able to perform UCCSD(T) or even UCCSDT(Q) computations. These results show that despite the fact that the unitary coupled cluster works very well within active space selection for some molecules, this is not always the case. The results could probably be improved with more qubits/larger active space selection and/or adding triple excitations. Future works will provide enhanced accuracy by improving the QLM simulator (i.e. by increasing the number of qubits). It is worth pointing out that an analysis for some molecules comparing the classical methods to UCCSD was previously studied in references. [18, 19]

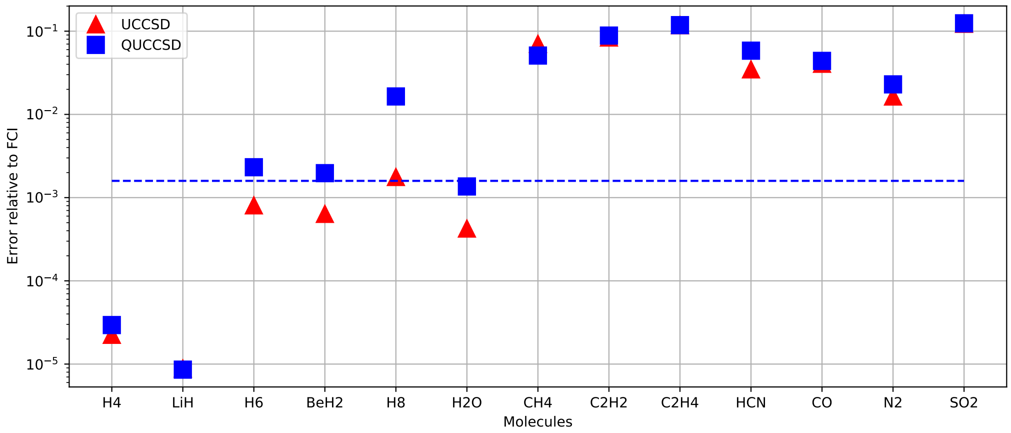


**(a)** UCCSD and QUCCSD methods.

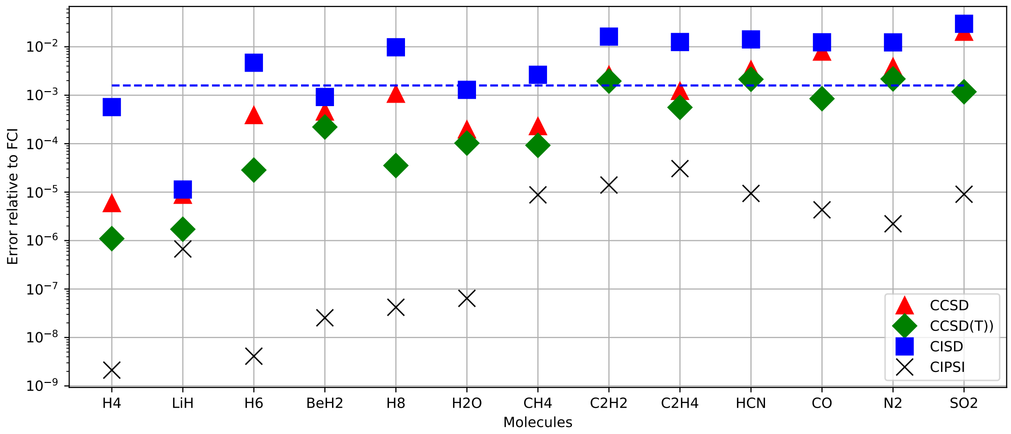


**(b)** CCSD, CCSD(T), CISD and CIPSI methods.

**Fig. S4.** Error, $(E - E_{FCI})$ in Hartree, from (a) UCCSD and QUCCSD, (b) CCSD, CCSD(T), CISD and CIPSI method calculations for a range of molecules with near equilibrium geometries. The basis set is STO-3G and all molecules are within a spin singlet state. (c) CNOT gates counts for UCCSD and QUCCSD after optimization (using MP2 Guess). Molecules $CH_4$, $C_2H_2$, $C_2H_4$, HCN, CO, $N_2$ and $SO_2$ are within active space selections (see text above). The dashed blue line indicates the chemical accuracy.

In Figure S5, we roughly estimate the number of CNOT gates found with UCCSD and QUCCSD ansätze for all the molecules listed above. We are interested in counting these gates because they are now the most critical required resources in the NISQ devices. Using our code function to count CNOT gates, we obtained very good count reductions. For example, for LiH, the number of CNOT gates decreased from 6976 to 4720 with the UCCSD ansatz (before and after the initial MP2 guess and subsequent optimization) and to (1112) with the QUCCSD ansatz. For $BeH_2$ molecule, it decreased from 18208 to 6368 with UCCSD (before and after the initial MP2 guess and subsequent optimization) and to (2592) with QUCCSD. We notice that in some molecules the CNOT count is reduced by around one-half between the UCCSD and QUCCSD ansätze.
Furthermore, for some other molecules within the active space selection approximation such as $C_2H_2$, $SO_2$, $CH_4$, and $C_2H_4$, the final CNOT counts with UCCSD and QUCCSD are about the same. We can conclude that QUCCSD exhibits lower gate counts, as compared to QLM's UCCSD,

due to its qubit evolutions construction. These CNOT gates counts with UCCCSD and QUCCSD have been previously studied for LiH, $H_6$ and $BeH_2$ in [20](see Table 3.1 in Chapter 4).

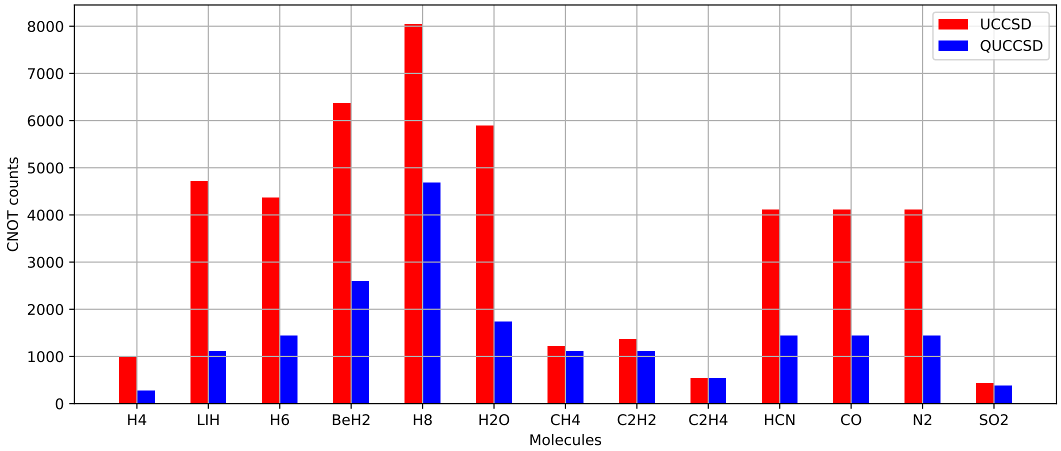


**Fig. S5.** CNOT gates counts for UCCSD and QUCCSD after optimization (using MP2 Guess), such that optimized parameters $\leq 10^{-8}$ are not counted.

### C. Fermionic-ADAPT-VQE: Simulating several Molecules Up to 22 Qubits: Basis sets, Comparison of Active and Non-active Space Selection

In this subsection, using the OpenVQE fermionic-ADAPT-VQE sub-module, we simulate a set of molecules (from 12 qubits up to 22 qubits) without active space selections with different basis sets. As mentioned in section 2.2 in the main text, the fermionic-ADAPT-VQE is based on excitation pool operators that are formed as spin-complement pairs of single and double fermionic evolutions. Spin-complement pair can be described as follows. It is a method that involves excitations that can preserve spin-symmetry for neutral closed-shell molecules (i.e number of $\alpha$ electrons = number of $\beta$ electrons). These excitations restrict the spin-symmetry of the UCC wavefunction Hilbert space into a smaller Hilbert space with the desired eigenstate. In order to satisfy such spin-symmetry, only the excitations that keep balance between $\alpha$ and $\beta$ electrons should be implemented as follows:

$$\tau_1 = (c^{\dagger}_{p_\alpha} c_{q_\alpha} - c^{\dagger}_{q_\alpha} c_{p_\alpha}) + (c^{\dagger}_{p_\beta} c_{q_\beta} - c^{\dagger}_{q_\beta} c_{p_\beta}). \tag{S1}$$

$$\begin{aligned}
\tau_{2,A} &= (c^{\dagger}_{r_\alpha} c_{s_\alpha} c^{\dagger}_{p_\alpha} c_{q_\alpha} - c^{\dagger}_{q_\alpha} c_{p_\alpha} c^{\dagger}_{s_\alpha} c_{r_\alpha}) + (c^{\dagger}_{r_\beta} c_{s_\beta} c^{\dagger}_{p_\beta} c_{q_\beta} - c^{\dagger}_{q_\beta} c_{p_\beta} c^{\dagger}_{s_\beta} c_{r_\beta}). \\
\tau_{2,B} &= (c^{\dagger}_{r_\alpha} c_{s_\beta} c^{\dagger}_{p_\alpha} c_{q_\beta} - c^{\dagger}_{q_\beta} c_{p_\alpha} c^{\dagger}_{s_\beta} c_{r_\alpha}) + (c^{\dagger}_{r_\beta} c_{s_\alpha} c^{\dagger}_{p_\beta} c_{q_\alpha} - c^{\dagger}_{q_\alpha} c_{p_\beta} c^{\dagger}_{s_\alpha} c_{r_\beta}). \\
\tau_{2,C} &= (c^{\dagger}_{r_\alpha} c_{s_\beta} c^{\dagger}_{p_\beta} c_{q_\alpha} - c^{\dagger}_{q_\alpha} c_{p_\beta} c^{\dagger}_{s_\beta} c_{q_\alpha}) + (c^{\dagger}_{r_\beta} c_{s_\alpha} c^{\dagger}_{p_\alpha} c_{q_\beta} - c^{\dagger}_{q_\beta} c_{p_\alpha} c^{\dagger}_{s_\alpha} c_{r_\beta}).
\end{aligned} \tag{S2}$$

This type of fermionic excitations is called spin-complemented pair: as is seen above in (Eqs. S1 and Eqs. S2), for each unitary operator acting on some spin orbitals, there is an added parallel unitary operator that acts on the opposite-spin orbitals. By implementing these equations in ADAPT-VQE sub-module, we were able to simulate small molecules as shown in section 5.3 in the main text. Moreover using the same ADAPT-VQE fermionic excitations, we simulated larger molecules. These molecules are: (i) with the STO-3G basis set: $OH^-$ (12 qubits), HF (12 qubits), $H_2O$ (14 qubits), $BeH_2$ (14 qubits), $NH_3$ (16 qubits) and $H_8$ (20 qubits); (ii) with the 6-31G basis set: $H_4$ (16 qubits) and LiH (22 qubits); (iii) in cc-pVDZ, $H_2$ (20 qubits). The goal in this subsection is to compare both the fermionic-ADAPT-VQE energies of these molecules affected by

an $\epsilon$ threshold value as well and the efficiency of our simulator.

Figure S6(a) shows the energy error convergence plots for the following set of molecules controlled by a given value of $\epsilon$: (i) $NH_3$ and $H_8$ ($\epsilon \leq 10^{-1}$), (ii) $BeH_2$ ($\epsilon \leq 10^{-2}$); (iii) $H_4$ and LiH ( $\epsilon \leq 10^{-3}$); (iv) $OH^-$, HF, $H_2$ and $H_2O$ ( $\epsilon \leq 10^{-5}$). We also observe in the Figure,that $H_2$ (cc-pVDZ) and $OH^-$ or HF (STO-3G) exhibit a precision superior to $10^{-8}$ (Ha) which is not the case for $H_4$ and LiH (6-31G) since the ADAPT-VQE loop stops at the given threshold (i.e. $\epsilon \leq 10^{-3}$). We also observe from the same Figure that even with $H_2O$, with the highest number of qubits (14 qubits) and a stopping threshold of $\epsilon \leq 10^{-5}$, we obtained a very good accuracy as the error being less than $10^{-6}$ Ha. Indeed, it is known from the literature, that as the threshold decreases, the chemical accuracy is improved regardless of the choice of basis sets. To illustrate this point (see Figure S7), we present detailed ADAPT-VQE calculations of the $H_2$ molecule using the cc-pVDZ basis set, showing that controlling $\epsilon$ at $10^{-4}$ brings very good accuracy (i.e. around $10^{-9}$ Ha) with respect to FCI(cc-pVDZ). For some molecules, we realized that some convergence problems might appear at certain levels of accuracy using fermionic-ADAPT-VQE especially when the size of molecules gets larger while including enough number of electrons. A similar study has been done for other sets of molecules in [21] where authors used Qiskit's state-vector simulator. They already mentioned the difficulty of fermionic ADAPT-VQE method in reaching certain convergence especially when $\epsilon$ gets too small i.e less than $10^{-4}$, in this paper it is suggested that choosing several maximum gradients (like 3 or 4) at each iteration instead of one maximum gradient can improve the convergence and reduce the number of iterations. Following this hypothesis, we are currently testing some larger molecular sizes in order to investigate how could the number of iterations, parameters and CNOTs could reduce instead of considering only one maximum gradient per external iteration in the ADAPT algorithm.

We also tested the fermionic-ADAPT submodule on a number of molecules using active space selection. The following molecules were simulated: (i) in STO-3G, $OH^-$ (10 qubits), LiH (10 qubits), $H_2O$ (12 qubits), $NH_3$ (14 qubits; (ii) in 6-31G, LiH (20 qubits). When we fixed the threshold ($\epsilon \leq 10^{-3}$), we observe in Figure S6 (b) that even with a reduction of qubits by 2 for each molecule, the accuracy is still present. Similarly to the non-active selection case, the threshold value of fermionic ADAPT-VQE must decrease in order to obtain better chemical accuracy. However, a good sign is that with qubit reductions, the fermionic ADAPT-VQE algorithm remains functional. This reduced the number of operators in the pool and thus the cost of gradient measurements. In a near future, we want to test molecules which require high numbers of qubits and to go beyond the STO-3G basis set ($CO_2$ or $C_2H_4$, benzene etc...) using the active space selection approximation. Such benchmarks are intended to check whether the performance of fermionic ADAPT-VQE from the QLM simulator is still working efficiently as the molecule size gets larger, especially with maintaining the level of accuracy.

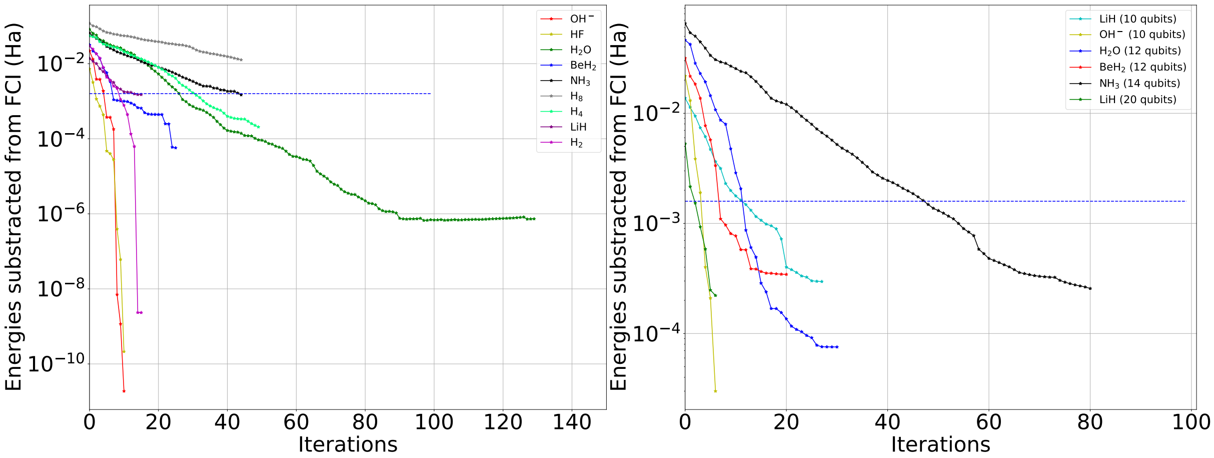


**(a)** No active space selections **(b)** Active space selections

**Fig. S6.** Fermionic ADAPT VQE simulations for a set of molecules ranging between 12 and 22 qubits. Iterations were stopped based on a given norm threshold condition. Subfigure (a) shows the error of energy for a set of molecules that are all assumed with full space selections and the STO-3G basis set for $OH^-$, $H_2O$, $BeH_2$, $NH_3$ and $H_8$, with 6-31G for $H_4$ and LiH, with cc-pVDZ for $H_2$. Subfigure (b) shows the error of the energy for a set a of molecules all assuming active space selections to tapper-off 2 qubits for each of the following molecules: in STO-3G for $OH^-$, $H_2O$, $BeH_2$, $NH_3$, with 6-31G for LiH. The dashed blue lines indicate the chemical accuracy.

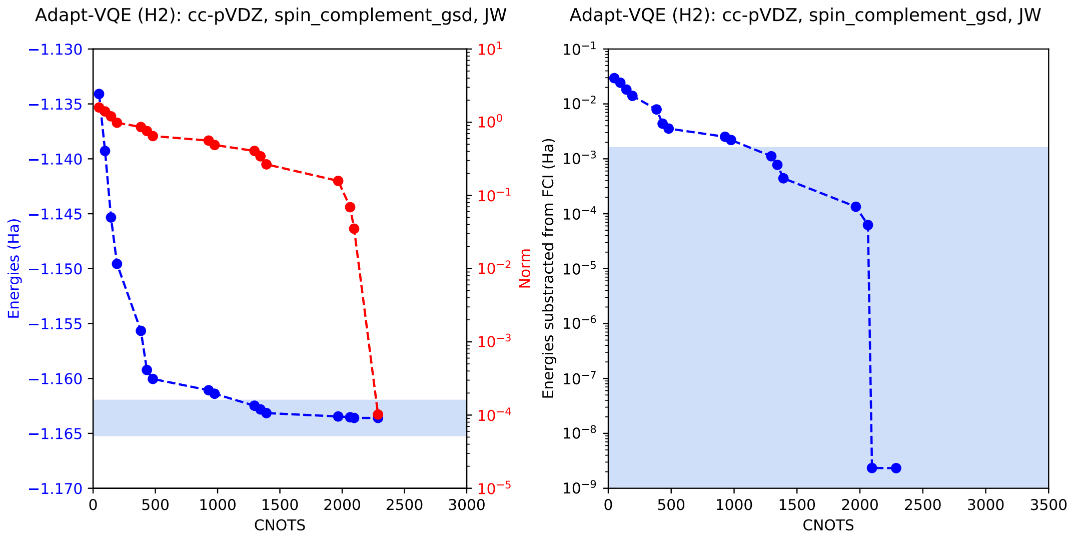


**(a)** Energy (Ha), Norm thresholds (red) as a function of
CNOT gates

**(b)** Error for the ground state energy given in subfigure(a) w.r.t FCI(cc-pVDZ) basis set

**Fig. S7.** Fermionic ADAPT VQE simulations in $H_2$ molecule (20 qubits) in cc-pVDZ basis set. Iterations were stopped based on a given norm threshold condition (which stops here at $10^{-4}$). The blue area represent the chemical accuracy.

### D. Qubit-ADAPT-VQE: Testing Several Qubit Pools

We study here in detail the qubit-ADAPT-VQE by providing an example of $H_4$ molecule at $r = 0.85$Å. In this molecule we test different qubit pools choices applying different pool sizes. We performed such simulations to understand which pool could achieve: i) a satisfying precision

with fewest iterations and CNOTs counts, ii) a reduced computational cost in term of gradients evaluation. We choose the first qubit pool by breaking down the spin-adapted fermionic operators[1], obtained after JW transformation and we choose the individual Pauli strings[2] which constructs the pool. Each individual Pauli string has the form

$$Q_m \equiv i\Pi_i p_i,\ p_i \in X, Y, Z \tag{S3}$$

and we named this qubit pool collecting $Q_m$ as *full*. It is obvious that this pool would yield larger sizes because it includes a large number of Pauli strings which consequently lead to a large number of CNOTs. A way to reduce the number of CNOTs and the pool size is to omit the $Z$ Pauli terms from *full*, which we named as *full_without_Z*. We can further reduce the pool by keeping the first string acting on each combination of spin orbitals named as *reduced_without_Z*[3]. Another possibility to test how the pool size behaves is to choose one type of the following strings[4] (*YXXX, XYXX, XXYX, XXXY*) and discarding their counter parts[5]. It appears that *reduced_without_Z* pool is the same as $YXXX$ pool operators at least for $H_4$ but not necessarily for other molecules with larger number of qubits. Randomly selecting operators from ($YXXX$, $XYXX$, $XXYXandXXXY$) and creating a pool mix out of them is named *Random*. Another possibility for checking the chemical accuracy and the number of iterations from the qubit-ADAPT-VQE ansatz is to group these Pauli strings into two or four qubit pools. We finally introduce a pool related to $H_4$ named *symmetry* (see [22], given in Eq. (11) therein). Very interesting, this pool contains the smallest number of operators[6], complete and minimal, preserving symmetry to avoid convergence problems. To do this test on our simulator, we use OpenVQE[7] to simulate the $H_4$ molecule by applying the qubit-ADAPT-VQE sub-module within the different pool size choices described above. For optimizing the search through the hyper-parameter space of rotations of quantum gates we choose the SLSQP algorithm with the energy convergence threshold of $10^{-13}$ (Ha).

Figure S8(a) presents the energy convergence plots with respect to FCI for each of the qubit pools. We observe that all these pools reach a an accuracy better than $10^{-8}$ Ha. We also observe that the $XXYX$ Qubit pool provides an accuracy above $10^{-10}$ Ha (convergence problems were observed)[8]. Other qubit pools yield an accuracy between $10^{-10}$ and around $10^{-12}$ Ha. Even though *full* and *four* pools reach comparable accuracy as that of *symmetry*, we observe no convergence problems with the latter since the *symmetry* pool preserves the *parity* symmetry, which is a property that other pools can miss. Our results are similar to those provided in [23] where some pool reduction simulation studies were analyzed for the $H_4$ and LiH molecules. Concerning the *symmetry* pool, a detailed analysis of this pool for the case of the $H_4$ molecule is given in Reference [22], but researchers there have performed their calculations analytically (i.e the exponential matrix of $Q_m$ is calculated by using *scipy.linalg.expm($Q_m$)* method[24]). Here we use the CNOT staircase method that map the exponential of Pauli strings found in the pool using QLM simulator. A comparison of our results in Figure S8 (a) to Figure 3 (b) found in[22]) illustrates that the QLM produces results similar as those of the analytical calculations. Figure S8 (b) shows the number of CNOT gates, the number of iterations needed to implement the ansatz and the size of each pool.

As is seen in Figure S8 (b), the *symmetry* pool requires higher number of CNOTs and iterations for completing an ansatz compared with some other pools at this level of accuracy. The *symmetry* pool still exhibits the lowest pool size (11 operators) which obviously helps a lot in reducing the cost of gradient energy measurements. Furthermore to construct the symmetry pools we can follow a recent work (see [22]). In this reference, $H_4$, LiH (18 operators) and $BeH_2$ (22 operators)

---

[1] The singlet generalized single and double excitation operators is considered which since we already used it in OpenVQE.

[2] the individual Pauli string in any qubit pool listed here has an important property: it contains an odd number of $Y$s because the fermionic operators are real. To make the final string real, it is multiplied by an imaginary part ($i$), however strings of even numbers of $Y$s cannot be considered because they don't affect the energy gradient

[3] YXXX strings comes always the first, because of internal organization from QLM/myQLM libray

[4] In the Jordan-Wigner transformation spin-up orbitals are mapped to even-numbered states and spin-down orbitals to odd-numbered states. This means that for the case of the single excitations (that act on qubits $i$ and $k$) we only keep the excitations that satisfy $i = k \pmod 2$, where mod denotes the modulo operation. Similarly, for the double excitations (that act on qubits $i, j, k, l$) we only keep that $i + j = k + l \pmod 2$.

[5] there are pairs of operators that are related by a global rotation, e.g., $Y_0X_1X_2X_3$ and $X_0Y_1Y_2Y_3$, so that we only need to keep one of them in the pool

[6] it scales linearly with the number of qubits (i.e 2n-2) according to [22]. This finding reduces the measurement cost from $O(n^8)$ to $O(n^5)$

[7] all Qubit pools are coded in Qubit Pool python class as discussed in subsection **??** and for the *symmetry* pool we followed the rules mentioned in [22] to classify which pool must be choosen as starters when we perform the loop of iterations

[8] Horizontal straight lines corresponds to poor convergences

are constructed by freezing one orbital per molecule which reduces the qubits counts: 10 for LiH and 12 for $BeH_2$ using the STO-3G basis set.

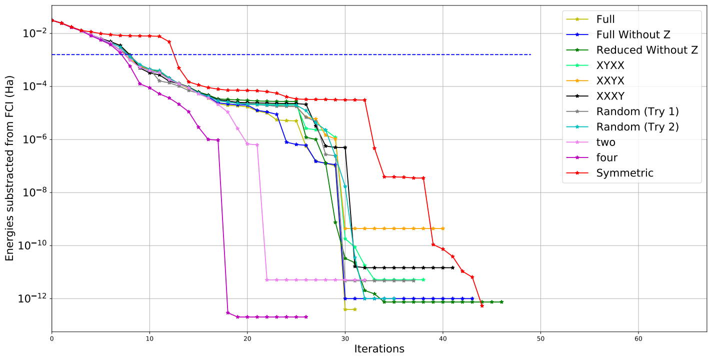


**(a)** Error for the ground state energy of the $H_4$ molecule (non-frozen: 8 qubits). The dashed blue line indicates the chemical accuracy.

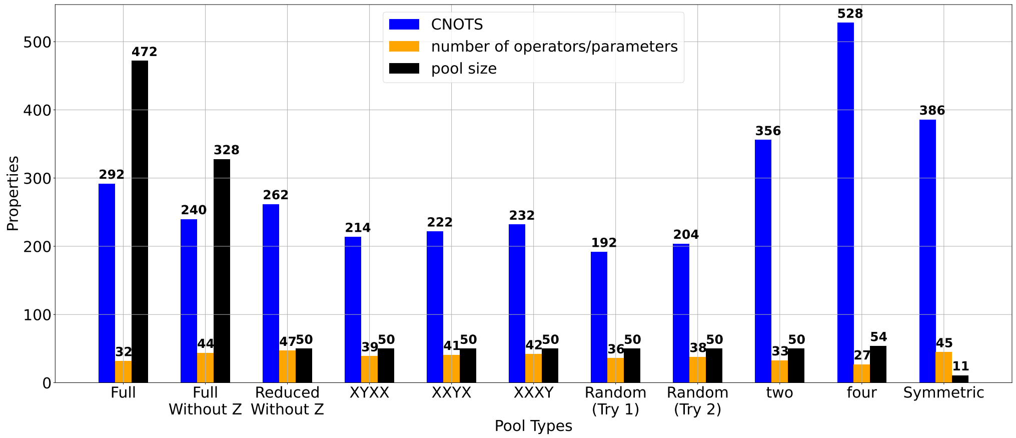


**(b)** Properties of qubit pools

**Fig. S8.** Qubit ADAPT-VQE: Graph (a) Energy error convergence of the $H_4$ molecule using the STO-3G basis set at $r = 0.85$Å for several kinds of qubit pools according to their arrangement: full, full without Z, reduced without Z, XYXX, XXYX, XXXY, Random with first try (Random Try1), and second Try (Random Try2), two, four, and pool preserves symmetry (symmetry), see text. Graph(b) shows for each pool type the following estimated three properties: the number of CNOT gates (CNOT), the number of parameters/operators, the size of each pool (pool size).

## REFERENCES


1. P.-F. Loos, Y. Damour, and A. Scemama, "The performance of cipsi on the ground state electronic energy of benzene," The J. Chem. Phys. **153**, 176101 (2020).
2. Y. Garniron, "Development and parallel implementation of selected configuration interaction methods," Ph.D. thesis, Université de Toulouse, Toulouse, France (2019).
3. "Quantum package: a programming environment for wave function methods," https://github.com/QuantumPackage/qp2, https://github.com/quantumlib/Cirq/graphs/contributors.
4. "myqlm package," https://myqlm.github.io/https://myqlm.github.io/.
5. "Interoperability with myqlm," https://myqlm.github.io/myqlm_specific/interoperability.htmlhttps://myqlm.github.io/*myqlm_specific*/interoperability.html.
6. S. McArdle, S. Endo, A. Aspuru-Guzik, S. C. Benjamin, and X. Yuan, "Quantum computational chemistry," Rev. Mod. Phys. **92**, 015003 (2020).
7. J. D. Whitfield, J. Biamonte, and A. Aspuru-Guzik, "Simulation of electronic structure hamiltonians using quantum computers," Mol. Phys. **109**, 735–750 (2011).
8. C. Hempel, C. Maier, J. Romero, J. McClean, T. Monz, H. Shen, P. Jurcevic, B. P. Lanyon, P. Love, R. Babbush *et al.*, "Quantum chemistry calculations on a trapped-ion quantum simulator," Phys. Rev. X **8**, 031022 (2018).
9. J. Romero, R. Babbush, J. R. McClean, C. Hempel, P. J. Love, and A. Aspuru-Guzik, "Strategies for quantum computing molecular energies using the unitary coupled cluster ansatz," Quantum Sci. Technol. **4**, 014008 (2018).
10. Y. S. Yordanov, V. Armaos, C. H. Barnes, and D. R. Arvidsson-Shukur, "Qubit-excitation-based adaptive variational quantum eigensolver," Commun. Phys. **4**, 1–11 (2021).
11. "Running gaussian," https://gaussian.com/running/https://gaussian.com/running/.
12. Y. Garniron, T. Applencourt, K. Gasperich, A. Benali, A. Ferté, J. Paquier, B. Pradines, R. Assaraf, P. Reinhardt, J. Toulouse, P. Barbaresco, N. Renon, G. David, J.-P. Malrieu, M. Véril, M. Caffarel, P.-F. Loos, E. Giner, and A. Scemama, "Quantum package 2.0: An open-source determinant-driven suite of programs," J. Chem. Theory Comput. **15**, 3591–3609 (2019). PMID: 31082265.
13. F. Lovas, E. Tiemann, J. Coursey, S. Kotochigova, J. Chang, K. Olsen, and R. Dragoset, "Diatomic spectral database," https://www.nist.gov/pml/diatomic-spectral-databaseDiatomic spectral database (2003).
14. G. Herzberg, *Electronic spectra and electronic structure of polyatomic molecules* (New York : Van Nostrand, 1966).
15. K.-P. Huber, *Molecular spectra and molecular structure: IV. Constants of diatomic molecules* (Springer Science & Business Media, 2013).
16. R. D. J. et al., "Nist computational chemistry comparison andbenchmark database, nist standard reference database number101 release 21," https://cccbdb.nist.gov/ (2020).
17. R. Xia and S. Kais, "Qubit coupled cluster singles and doubles variational quantum eigensolver ansatz for electronic structure calculations," Quantum Sci. Technol. **6**, 015001 (2020).
18. G. Harsha, T. Shiozaki, and G. E. Scuseria, "On the difference between variational and unitary coupled cluster theories," The J. chemical physics **148**, 044107 (2018).
19. M. Kühn, S. Zanker, P. Deglmann, M. Marthaler, and H. Weiß, "Accuracy and resource estimations for quantum chemistry on a near-term quantum computer," J. chemical theory computation **15**, 4764–4780 (2019).
20. Y. Yordanov, "Quantum computational chemistry methods for early-stage quantum computers," Ph.D. thesis, University of Cambridge, Cambridge, UK (2021).
21. S. Carrazza, S. Efthymiou, M. Lazzarin, and A. Pasquale, "An open-source modular framework for quantum computing," arXiv preprint arXiv:2202.07017 (2022).
22. V. Shkolnikov, N. J. Mayhall, S. E. Economou, and E. Barnes, "Avoiding symmetry roadblocks and minimizing the measurement overhead of adaptive variational quantum eigensolvers," arXiv preprint arXiv:2109.05340 (2021).
23. H. L. Tang, V. Shkolnikov, G. S. Barron, H. R. Grimsley, N. J. Mayhall, E. Barnes, and S. E. Economou, "qubit-adapt-vqe: An adaptive algorithm for constructing hardware-efficient ansätze on a quantum processor," PRX Quantum **2**, 020310 (2021).
24. P. Virtanen, R. Gommers, T. E. Oliphant, M. Haberland, T. Reddy, D. Cournapeau, E. Burovski, P. Peterson, W. Weckesser, J. Bright, S. J. van der Walt, M. Brett, J. Wilson, K. J. Millman, N. Mayorov, A. R. J. Nelson, E. Jones, R. Kern, E. Larson, C. J. Carey, İ. Polat, Y. Feng, E. W. Moore, J. VanderPlas, D. Laxalde, J. Perktold, R. Cimrman, I. Henriksen, E. A. Quintero, C. R. Harris, A. M. Archibald, A. H. Ribeiro, F. Pedregosa, P. van Mulbregt, and SciPy 1.0

Contributors, "SciPy 1.0: Fundamental Algorithms for Scientific Computing in Python," Nat. Methods **17**, 261–272 (2020).
